# Supplementary material for: ViVid-1-to-3: Novel View Synthesis with Video Diffusion Models
Source: arXiv:2312.01305 source file (2023-12-03)

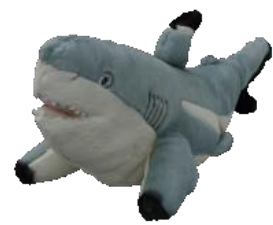

Input  
image

$F = 1$   
(Zero-1-to-3 XL)

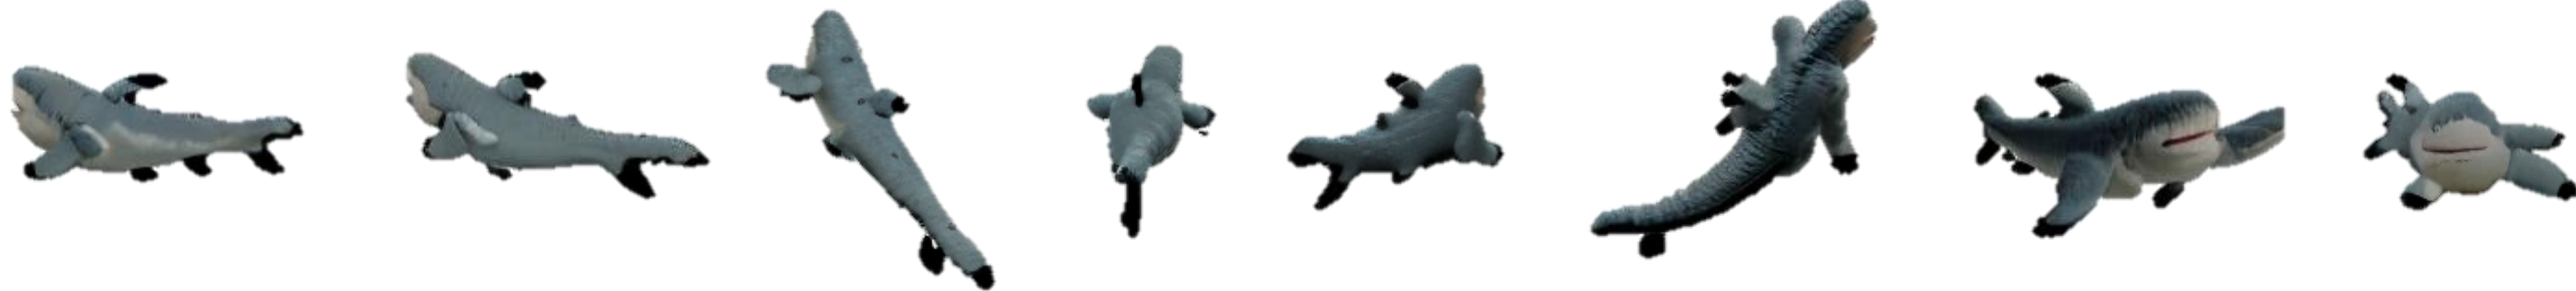

$F = 12$

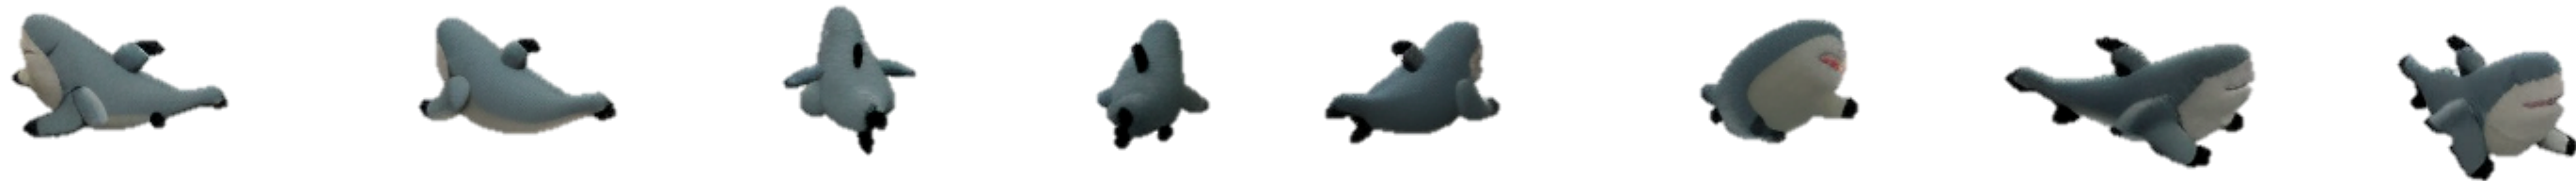

$F = 24$

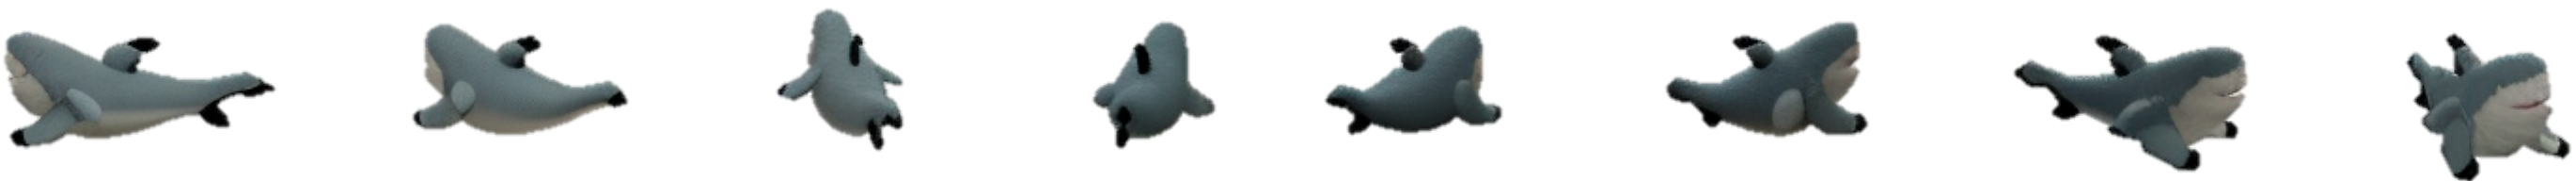

$F = 36$

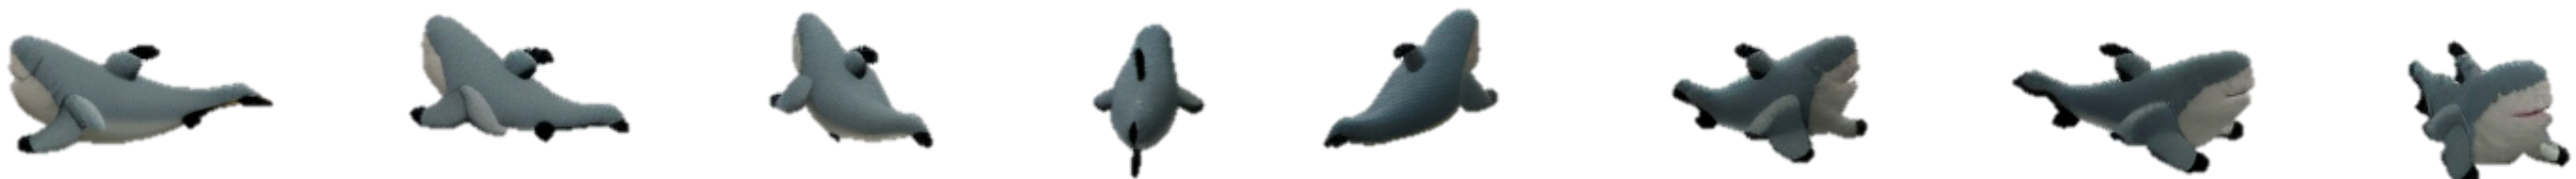

GT

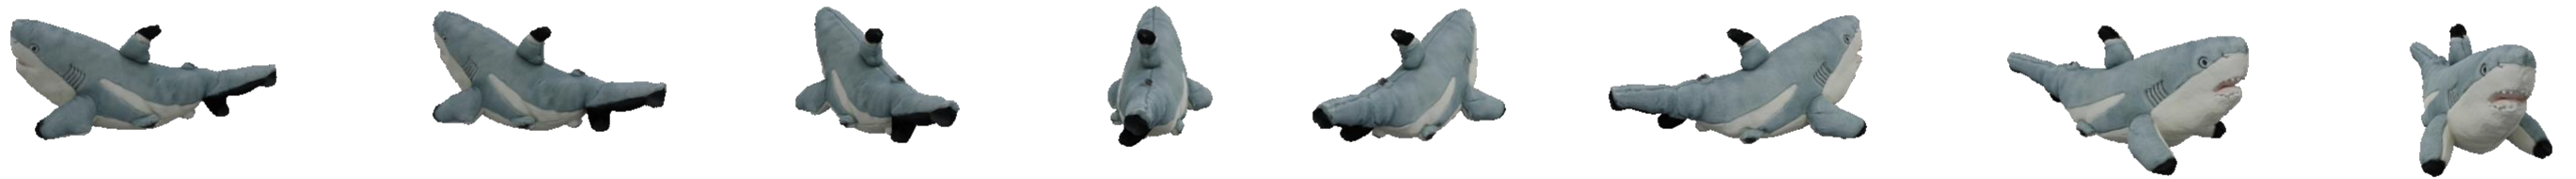

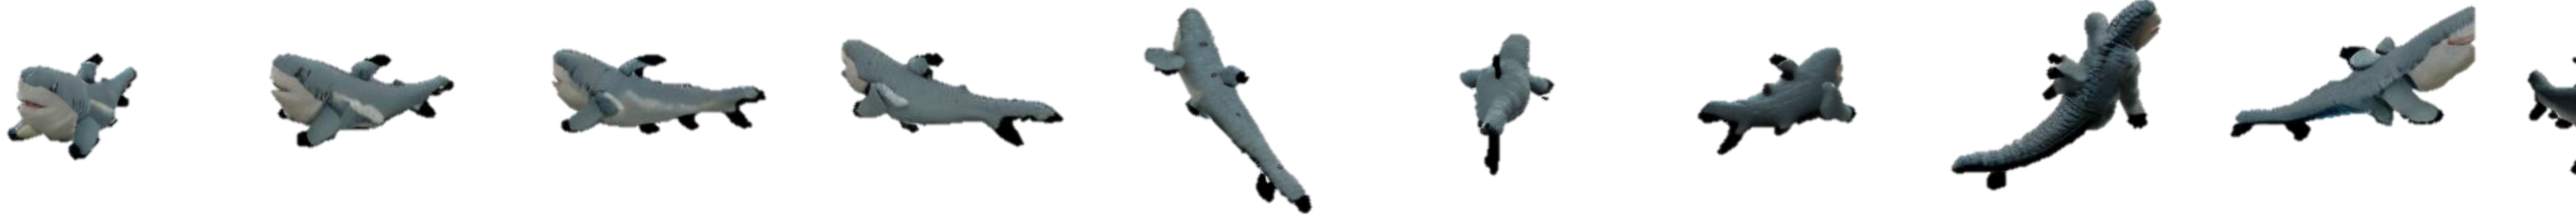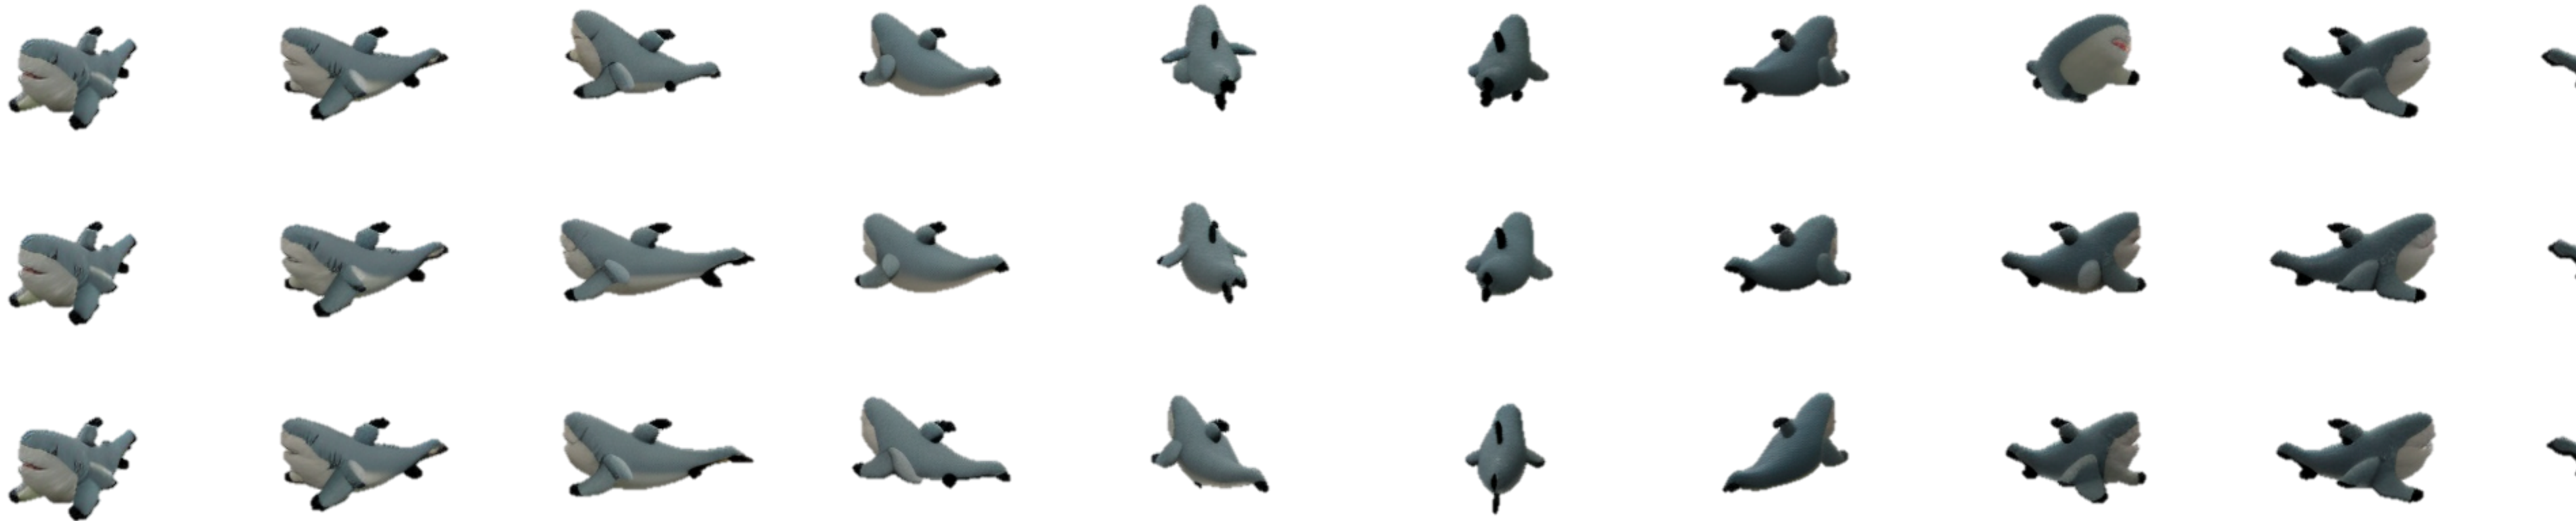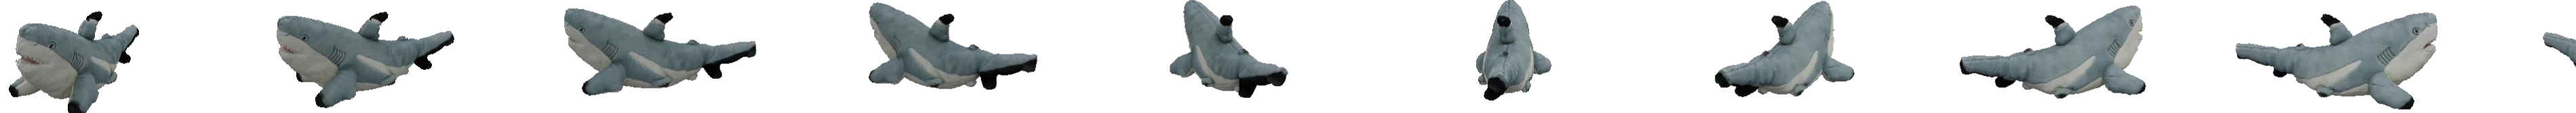

Supplement: Supplementary file 1 [file suppl_ablation_framenum.pdf]
