# Supplementary material for: ViVid-1-to-3: Novel View Synthesis with Video Diffusion Models
Source: arXiv:2312.01305 source file (2023-12-03)

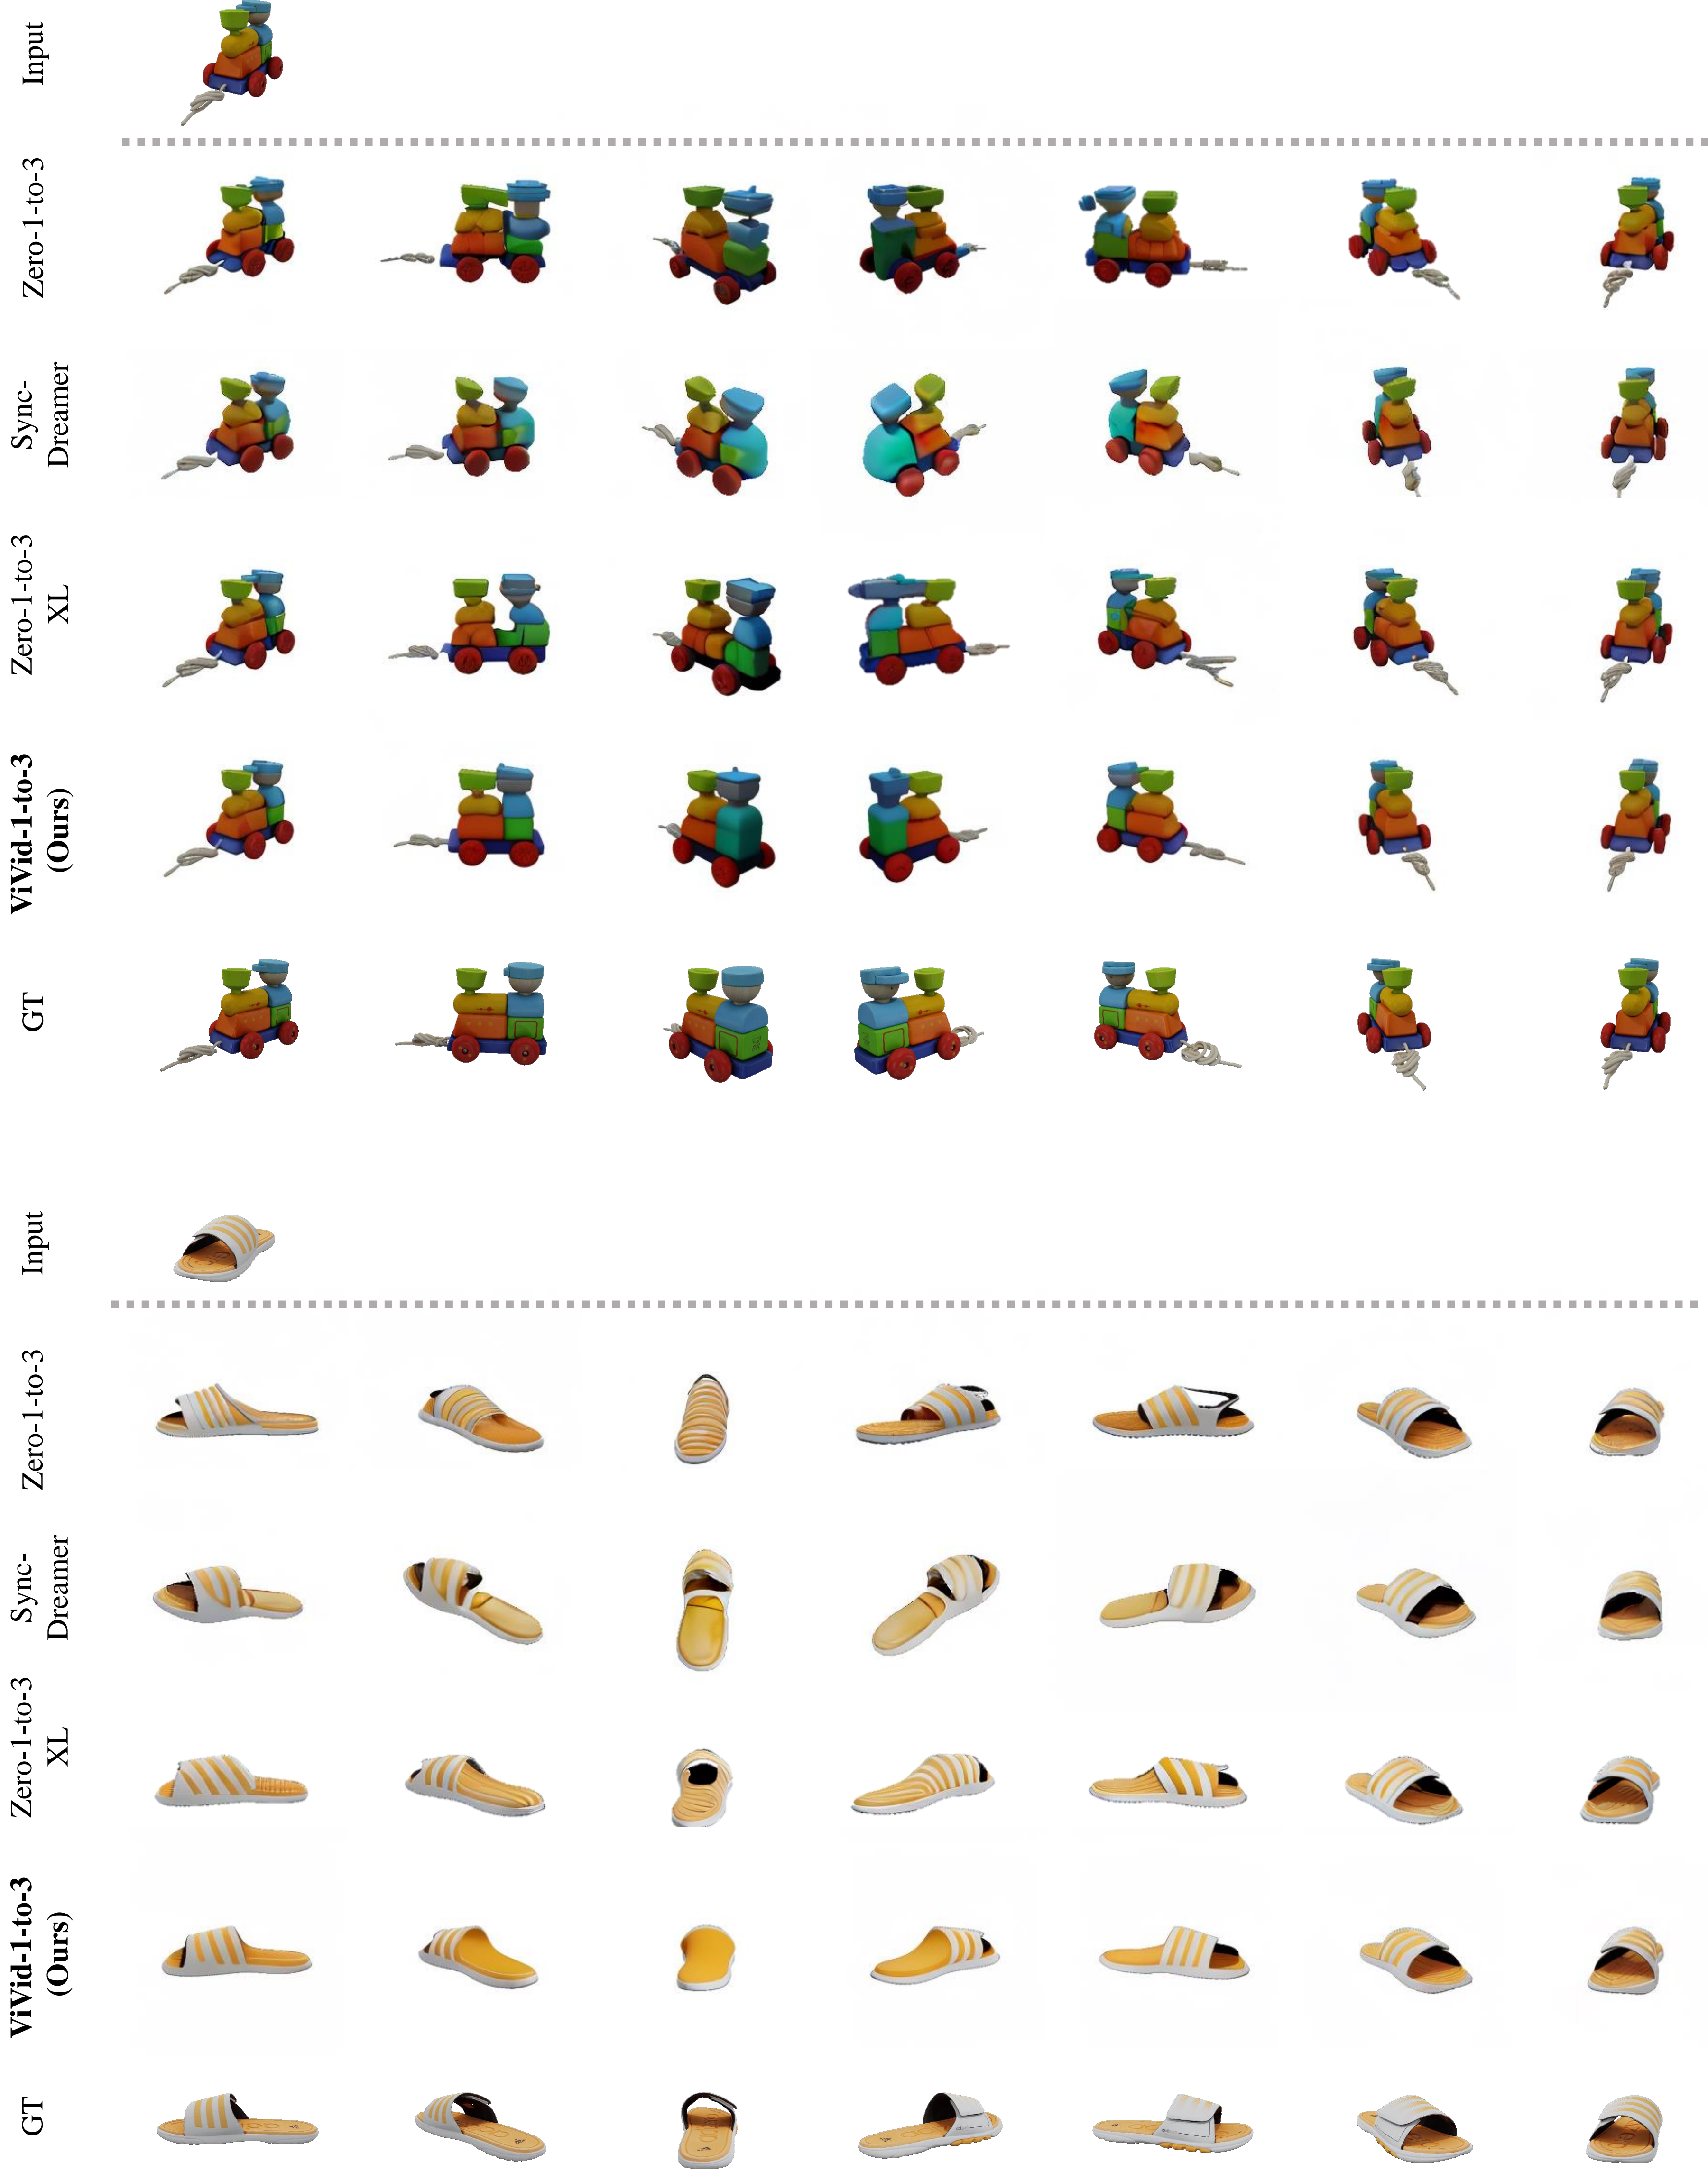



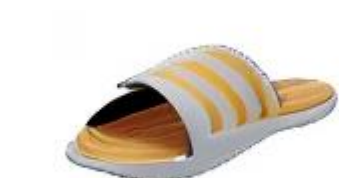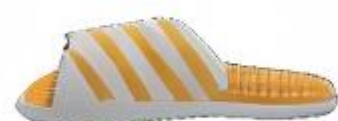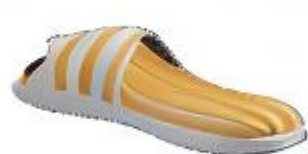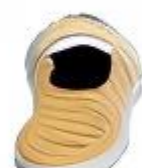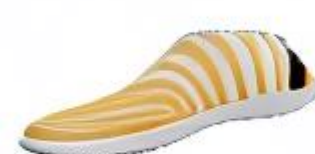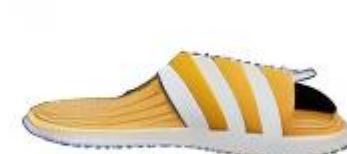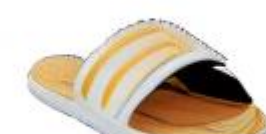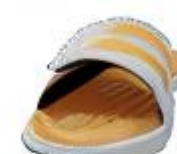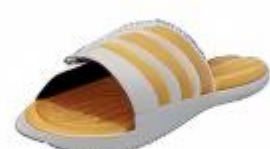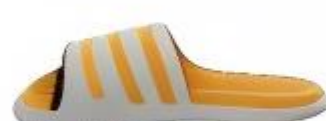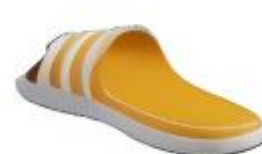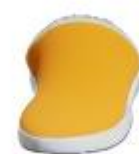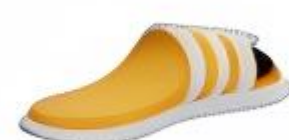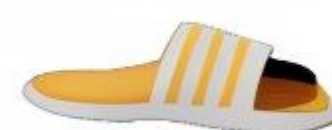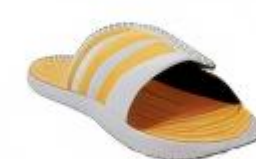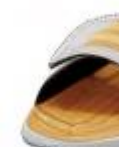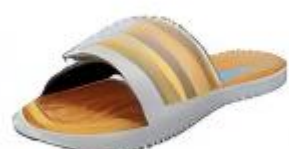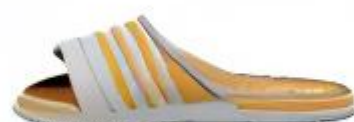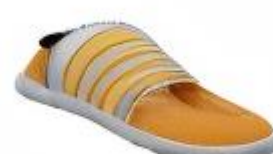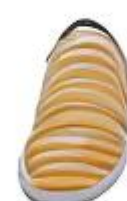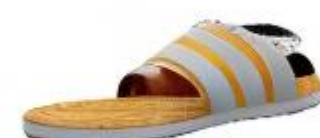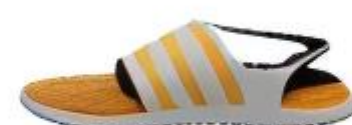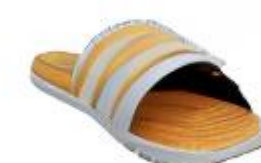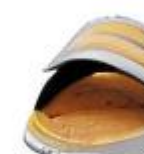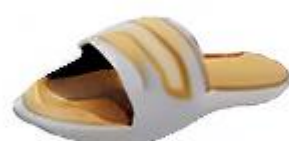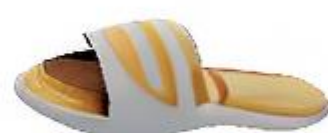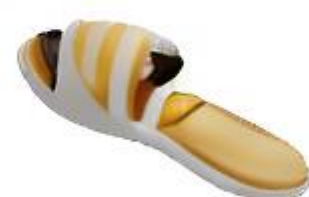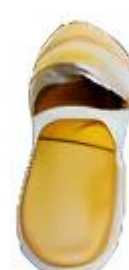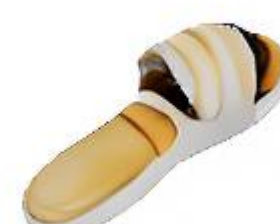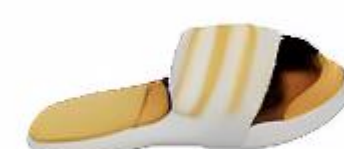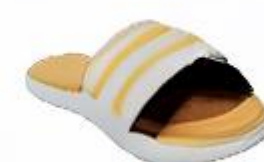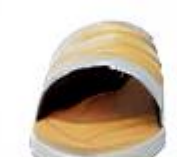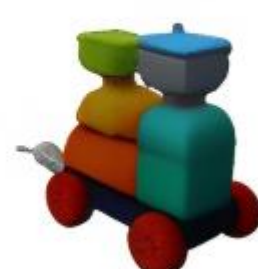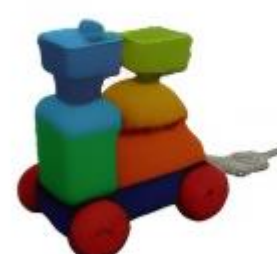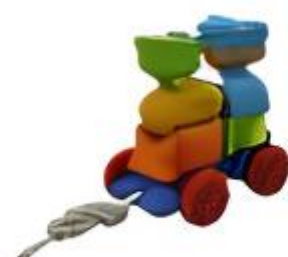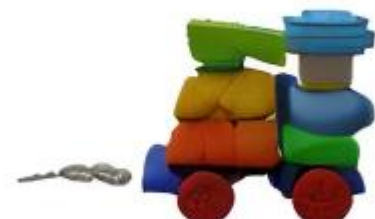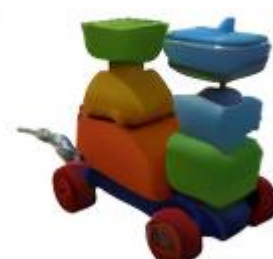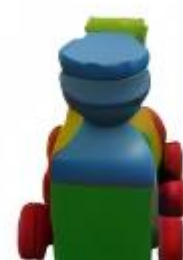



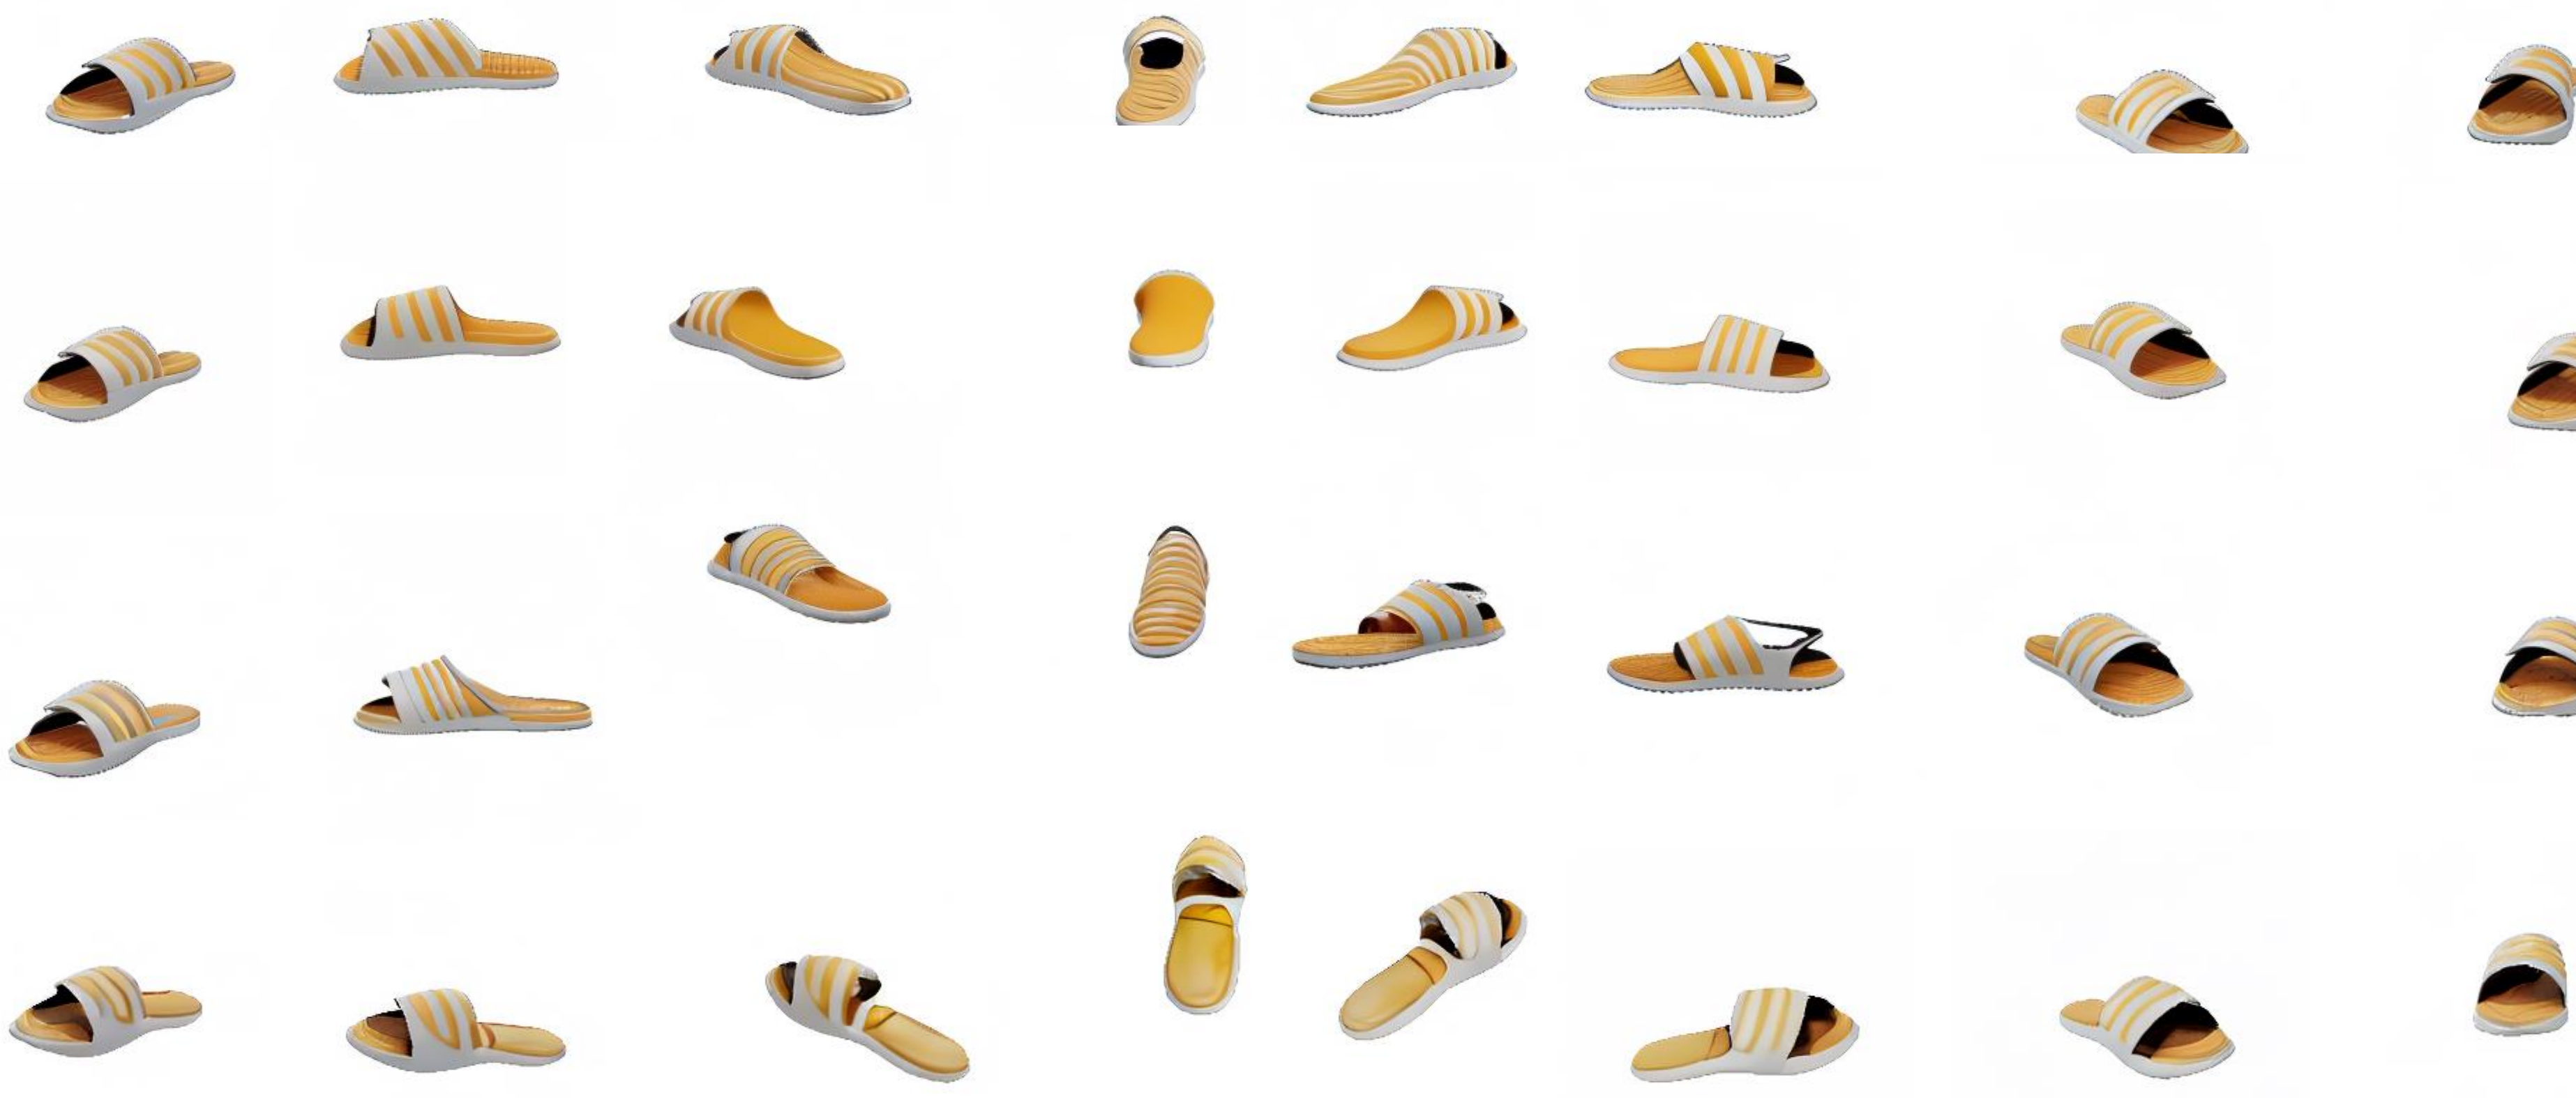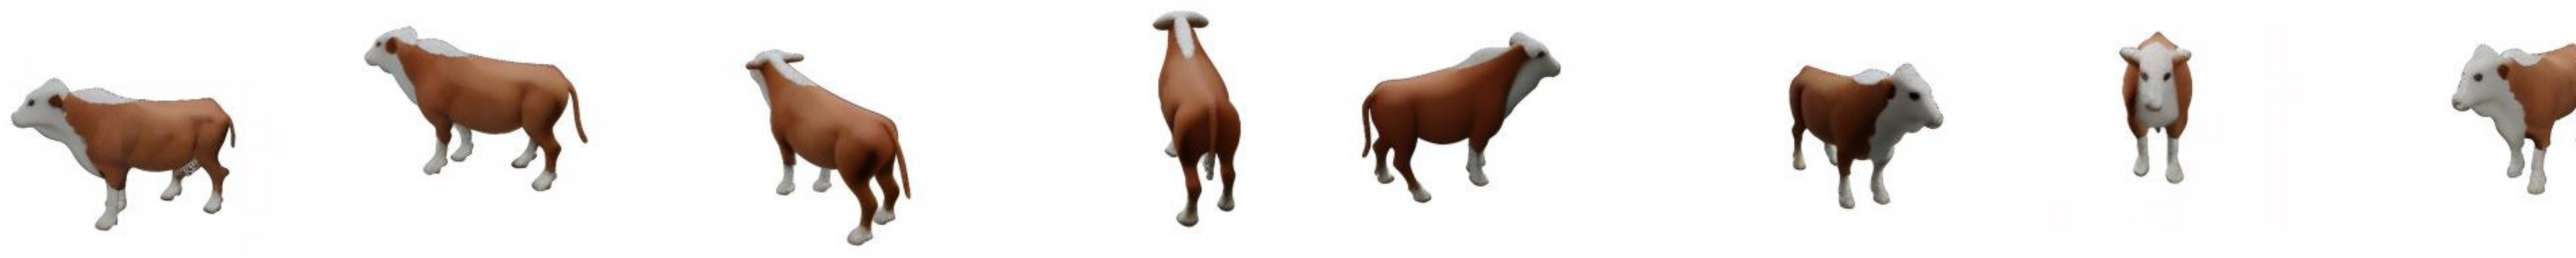

2, 4,6,8,12,18,20,22

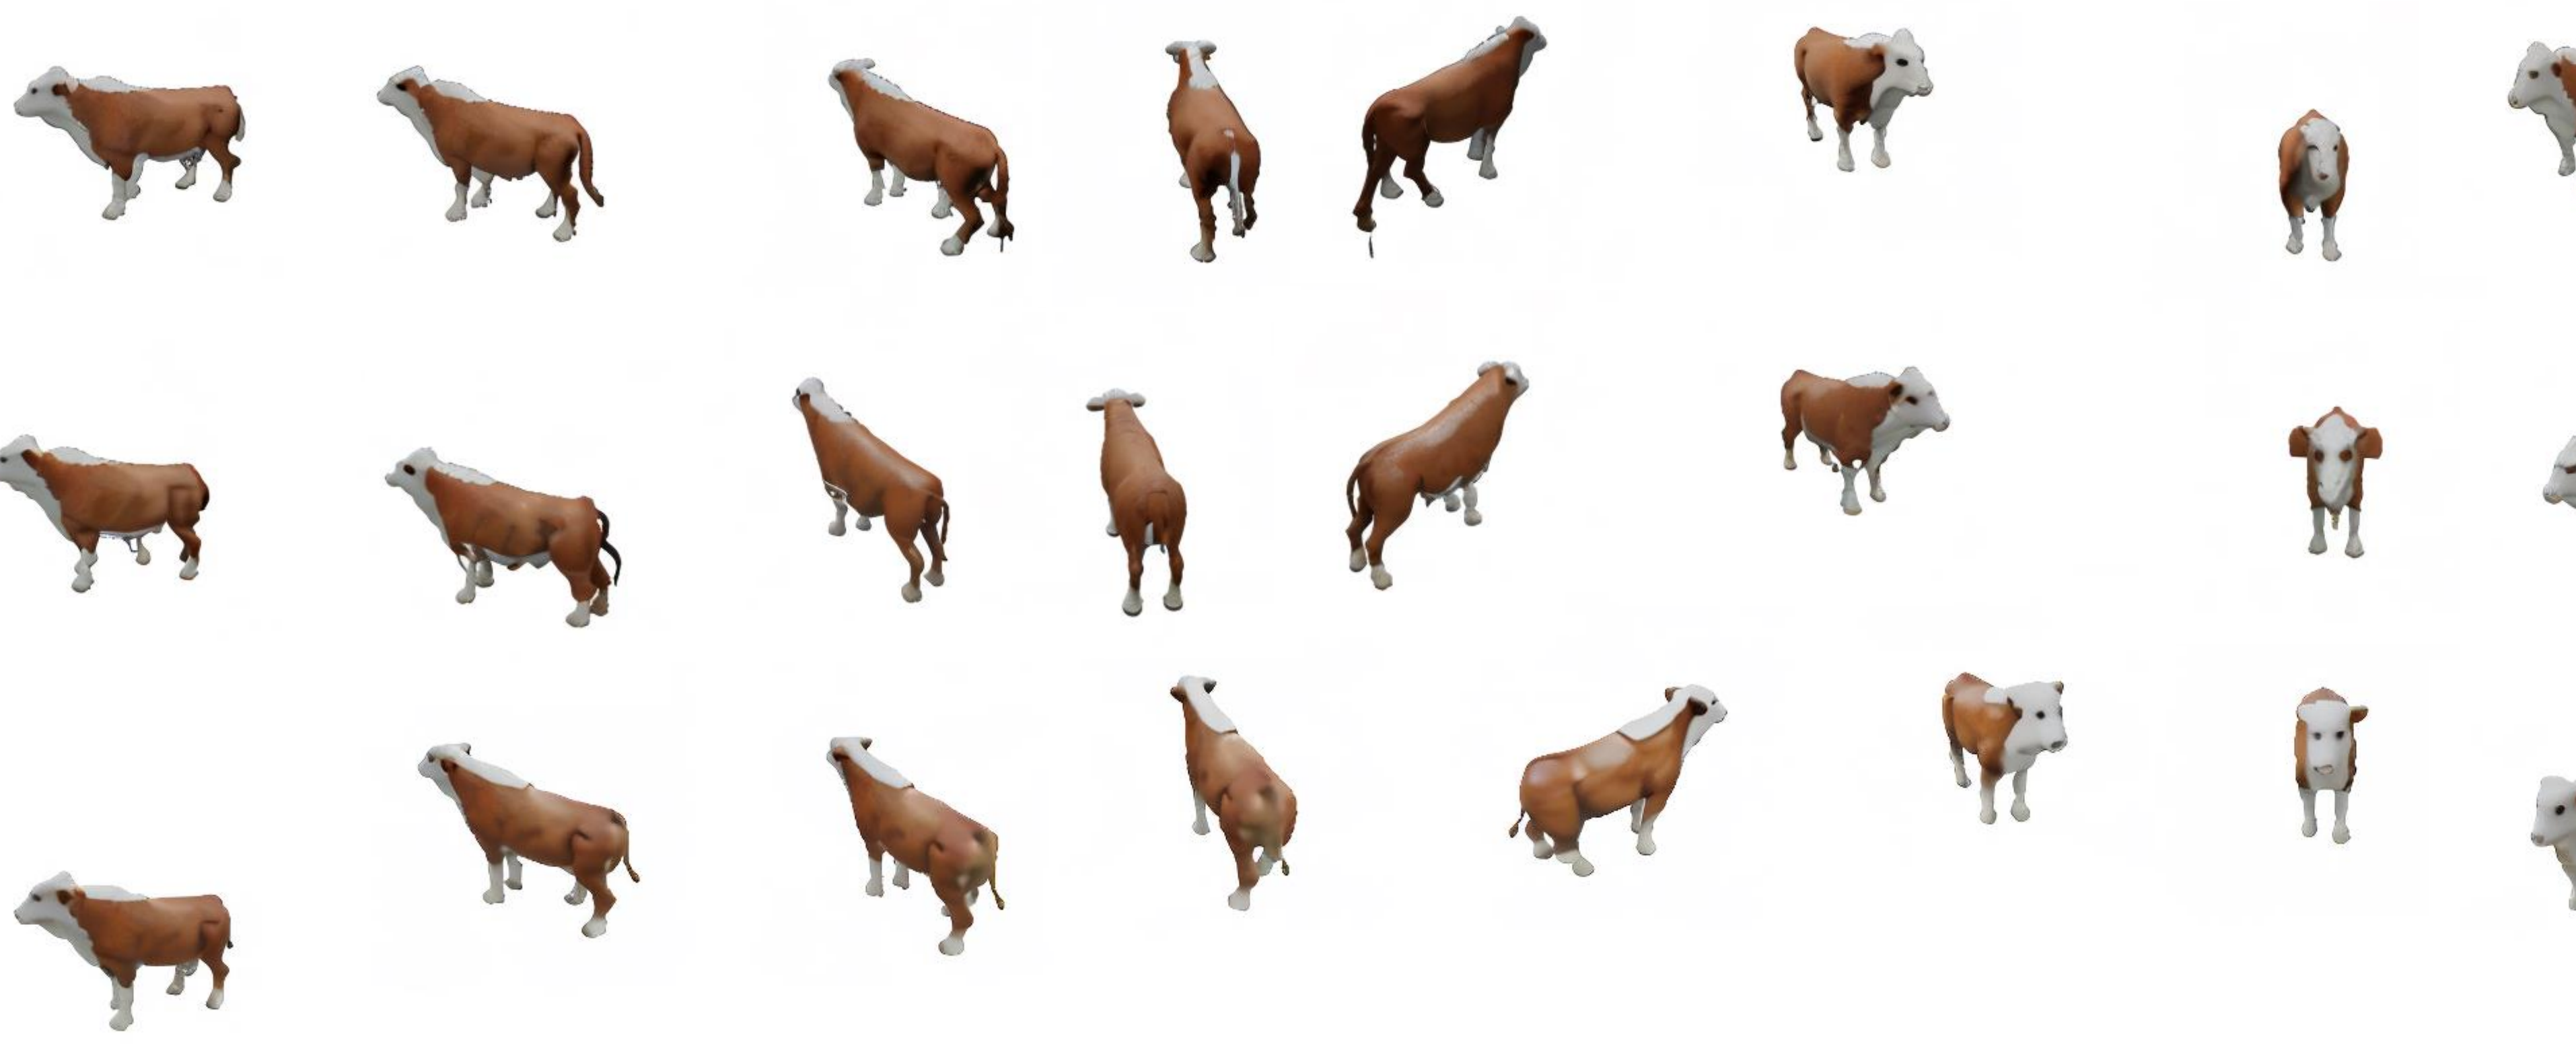

Supplement: Supplementary file 2 [file suppl_qual_vs_2d.pdf]
